# Supplementary material for: Equilibria for Games with Combined Qualitative and Quantitative Objectives
Source: arXiv:2008.05643 source file (2020-08-13)
Supplement: Supplementary file 1 [file appendix.tex]

\head{Push weights into the states}
	This is done by replacing $St$ by $St \times Act^{Ag}$ and defining the weight of $(s,d)$ to be $\kappa(d)$.
	Formally, we obtain a state-weighted arena $A' = (AG, Act, Ap, W, St', \iota', tr', \lambda, (\kappa'_{a})_{a \in Ag})$ with $\kappa'_a: St' \to W$, such that
	
	\begin{itemize}
		\item
			$St' = St \times Act^{Ag}$;
			
		\item
			$\iota' = (\iota, d)$ for some $d \in Act^{Ag}$;
			
		\item
			$\lambda'(s,d) = \lambda(s)$;
			
		\item
			$\kappa'_a(s,d) = \kappa_a(d_a)$;
			
		\item
			$tr'((s,d), d') = (tr(s,d'), d')$.
	\end{itemize}

	Games on state-weighted arenas are defined as before: simply note that one can extend $\kappa'_a$ to executions, 
	i.e., for $\pi = t_0 d_0 t_1 d_1 \dots$, define $\kappa'_a(\pi) = \kappa_a(t_0) \kappa_a(t_1) \cdots$.
	
	\begin{lemma}
		\label{lmm:ltltoparity}
		For every $\epsilon > 0$ and every \LEX(\buchi, \mp) game $G = (A, \Psi)$, it holds that $\NE^\epsilon(G) = \NE^\epsilon(A',\Psi)$.
	\end{lemma}
	
	\begin{proof}
		\todo{missing}
%		
%		By construction we have that $\NE(G) = \NE(G)$.
%	
%		Observe that $A$ and $A'$ have the same set of agents and action. Thus, due to Remark~\ref{rmk:actstrat} we can assume they have the same set of strategies.
%		It is not hard to see that a strategy profile is a Nash Equilibrium in  $G= (A, \Psi)$ if and only if it is so in $G = (A', \Psi)$ too.
	\end{proof}
	
	Thus, without loss of generality, we assume that $G$ has weights on the states.
